# Supplementary material for: Training-free steering of video diffusion models for functional object interaction
Source: arXiv:2611.41195 source file (2026-11-30)
Supplement: Supplementary file 2 [file authors.tex]

\author{
\begin{minipage}{0.19\textwidth}
    \vspace*{-7mm}
    \centering
    Jaime Corsetti$^{1,2}$
\end{minipage}
\begin{minipage}{0.19\textwidth}
    \vspace*{-7mm}
    \centering
    Francesco Giuliari$^1$
\end{minipage}
\begin{minipage}{0.19\textwidth}
    \vspace*{-7mm}
    \centering
    Davide Boscaini$^1$
\end{minipage}
\begin{minipage}{0.16\textwidth}
    \vspace*{-7mm}
    \centering
    Fabio Poiesi$^1$
\end{minipage} \\
\hfill
\begin{minipage}[t]{0.45\textwidth}
\centering
     $^1$Fondazione Bruno Kessler
\end{minipage}
\begin{minipage}[t]{0.45\textwidth}
\centering
    $^2$University of Trento
\end{minipage} \\
\hfill
}
