# Supplementary material for: Training-free steering of video diffusion models for functional object interaction
Source: arXiv:2611.41195 source file (2026-11-30)
Supplement: Supplementary file 3 [file mypackages.tex]

\usepackage{algorithmic}
\usepackage{array}
\usepackage{textcomp}
\usepackage{stfloats}
\usepackage{url}
\usepackage{graphicx}
\usepackage{amsmath,amssymb,amsfonts}
\usepackage{bbm}
\usepackage{multirow,multicol}
\usepackage[T1]{fontenc}
\usepackage[accsupp]{axessibility}
\usepackage{microtype}
\usepackage{balance}
\usepackage{wrapfig,booktabs}
\usepackage{overpic}
\usepackage{pifont}
\usepackage{tikz}
\usetikzlibrary{patterns}
\usepackage{pgfplots}
\usepackage{comment}
\usepackage{dsfont}
\usepackage[normalem]{ulem}
\pgfplotsset{compat=1.18}
\pgfplotsset{every axis/.append style={
    title={\small \textbf{Overall Preference}},
    title style={at={(0.5,1)}, anchor=south, yshift=0pt},
    ymin=0, ymax=100,
    ybar stacked, bar width=15pt,
    xtick=data,
    ytick={},
    yticklabels={},
    grid=major,
    major grid style={line width=0.3pt, gray!30},
    axis x line=bottom,
    axis y line=left,
    axis line style = {draw=none},
    x tick label style={rotate=0, anchor=north},
    enlarge x limits=0.35,
    nodes near coords={\pgfmathprintnumber{\pgfplotspointmeta}\%},
    every node near coord/.append style={font=\tiny, text=black},
    width=3cm, height=4cm,
    tick label style={font=\small},
}}

\usepackage{xcolor}
\definecolor{lightgraybg}{RGB}{245,245,245}
\definecolor{deepgrayborder}{RGB}{120,120,120}
\usepackage[table]{xcolor}
\definecolor{verylightpink}{HTML}{FFD6D6}
\definecolor{brightgreen}{RGB}{0,176,80}

\usepackage{listings}
\lstset{
    escapeinside={(*}{*)},
    breaklines=true, 
    breakatwhitespace=true, 
    breakautoindent=false,
    backgroundcolor=\color{lightgraybg}, 
    frame=single,
    rulecolor=\color{deepgrayborder}, 
    framerule=1.2pt, 
}

\usepackage{tabularx}
\usepackage{todonotes}
\usepackage{fontawesome5}



\usepackage{cuted}

\usepackage{currfile}

\usepackage{caption}
